# Supplementary material for: Multi-Modal Domain Adaptation Across Video Scenes for Temporal Video Grounding
Source: arXiv:2312.13633 source file (2023-12-21)
Supplement: Supplementary file 1 [file ethical.tex]

\section{Ethical Discussion}
Considering the potential application of the NLTVG task, such as video search engines and automated video editing, some offensive data could be used in real applications. However, in our experiments, the models are trained on well-collected datasets, which may not be directly applied to real practice.
